# Supplementary material for: TLP: A Deep Learning-based Cost Model for Tensor Program Tuning
Source: arXiv:2211.03578 source file (2022-11-22)
Supplement: Supplementary file 1 [file 11_appendix.tex]

\section{Experimental Result}\label{all_curve_appdix}
\input{asplos23/figs/6_1_curve_appendix}
